# Supplementary material for: Coherent spatial control of wave packet dynamics on quantum lattices
Source: arXiv:2311.07254 ancillary file (2023-11-13)
Supplement: Supplementary file 1 [file SI.pdf]

# Supporting Information for: Coherent spatial control of wave packet dynamics on quantum lattices

Ilia Tutunnikov,[1] Chern Chuang,[2] and Jianshu Cao[1,*]

[1]Department of Chemistry, Massachusetts Institute of Technology, 77 Massachusetts Avenue, Cambridge, Massachusetts 02139, USA
[2]Department of Chemistry and Biochemistry, University of Nevada, 4505 S Maryland Pkwy, Las Vegas, Nevada 89154, USA

This Supporting Information summarizes the derivations of various diffusivity formulae from the main text. In addition, it contains auxiliary figures to help the qualitative understanding of several points raised in the main text.

## CONTENTS

I. Derivation – diffusivity in an isolated system 1

II. List of spatial coherences 2
A. Standing Gaussian wave 2
B. Traveling Gaussian 2

III. Momentum representation 2
A. Gaussian initial state 2
B. Traveling Gaussian initial state 2

IV. Diffusivity through the Green-Kubo formula 3
A. Gaussian initial state 3
B. Traveling Gaussian initial state 3

V. Derivation – diffusivity in the presence of noise (HSR model) 4

References 4

## I. DERIVATION – DIFFUSIVITY IN AN ISOLATED SYSTEM

In this section, we detail the derivation of the diffusivity expressions in an isolated system. The definition of diffusivity, $D(t)$ reads

$$2D(t)=\frac{d\langle n^2(t)\rangle}{dt}-\frac{d\langle n(t)\rangle^2}{dt}, \tag{S1}$$

Starting with $d\langle n(t)\rangle/dt=\sum_n n\dot\rho_{n,n}(t)$, the derivative of the diagonal element of the density matrix $\dot\rho_{n,n}$ is obtained from $\dot\rho=-i[H,\rho]=-i(H\rho-\rho H)$, where $H$ is Hamiltonian matrix expressed in the basis of localized states. Assuming nearest-neighbor coupling, and using $\mathrm{Im}[\rho_{m,n}]=-\mathrm{Im}[\rho_{n,m}]$, we find

$$\begin{aligned}i\dot\rho_{n,n}(t)&=\sum_m H_{n,m}\rho_{m,n}(t)-\sum_m\rho_{n,m}(t)H_{m,n}\\&=J\sum_m(\delta_{m,n-1}+\delta_{m,n+1})(\rho_{m,n}-\rho_{n,m})\\&=J(\rho_{n-1,n}-\rho_{n,n-1}+\rho_{n+1,n}-\rho_{n,n+1})\\&=2iJ\mathrm{Im}[\rho_{n-1,n}+\rho_{n+1,n}].\end{aligned} \tag{S2}$$

Thus,

$$\frac{d\langle n(t)\rangle}{dt}=2J\sum_n n\mathrm{Im}[\rho_{n-1,n}+\rho_{n+1,n}]. \tag{S3}$$

The sum on the right hand side can be simplified by noticing the partial cancellation of the consecutive terms in the sum, such that

$$\frac{d\langle n(t)\rangle}{dt}=2J\sum_n\mathrm{Im}[\rho_{n,n+1}(t)]=2J\mathrm{Im}[\langle\rho(t)\rangle_1], \tag{S4}$$

where we used the following definitions ($l\geq 0$)

$$\langle\rho(t)\rangle_l=\sum_n\rho_{n,n+l}(t),\quad \langle n(t)\rangle_l=\sum_n n\rho_{n,n+l}(t). \tag{S5}$$

The expression for $d\langle n^2(t)\rangle/dt$ can be obtained similarly

$$\begin{aligned}\frac{d\langle n^2(t)\rangle}{dt}&=2J\sum_n n^2\mathrm{Im}[\rho_{n-1,n}+\rho_{n+1,n}]\\&=2J\sum_n[(n+1)^2-n^2]\mathrm{Im}[\rho_{n,n+1}]\\&=4J\sum_n n\mathrm{Im}[\rho_{n,n+1}]+2J\sum_n\mathrm{Im}[\rho_{n,n+1}]\\&=4J\mathrm{Im}[\langle n(t)\rangle_1]+2J\mathrm{Im}[\langle\rho(t)\rangle_1],\end{aligned} \tag{S6}$$

So far, the formulae are general and rely only on the nearest-neighbor coupling.

In the noise-free case, $\langle\rho(t)\rangle_1=\sum_n\dot\rho_{n,n+1}(t)$ appearing in Eqs. (S4) and (S6) is conserved. To prove that, consider

$$\begin{aligned}i\dot\rho_{n,n+1}(t)&=\sum_m H_{n,m}\rho_{m,n+1}-\sum_m\rho_{n,m}H_{m,n+1}\\&=J\sum_m(\delta_{m,n-1}+\delta_{m,n+1})\rho_{m,n+1}-\rho_{n,m}(\delta_{m,n+2}+\delta_{m,n})\\&=J(\rho_{n-1,n+1}+\rho_{n+1,n+1}-\rho_{n,n+2}-\rho_{n,n}),\end{aligned} \tag{S7}$$

and notice that the consecutive terms in the sum $\sum_n\dot\rho_{n,n+1}$ cancel out resulting in $d\langle\rho\rangle_1/dt=0$. Generally, in an isolated system, $d\langle\rho\rangle_l/dt=0$ for $l\geq 0$. The conservation of $\langle\rho\rangle_l$ allow us to solve the differential equation in Eq. (S4)

$$\langle n(t)\rangle=2J\mathrm{Im}[\langle\rho(0)\rangle_1]t+\langle n(0)\rangle. \tag{S8}$$

Next, we consider $\langle n(t)\rangle_1$ appearing in Eq. (S6)

$$\begin{aligned}\frac{d\langle n(t)\rangle_1}{dt}&=-iJ\sum_n n(\rho_{n-1,n+1}-\rho_{n,n}+\rho_{n+1,n+1}-\rho_{n,n+2})\\&=-iJ\sum_n(-\rho_{n-1,n+1}+\rho_{n,n+2})=iJ[1-\langle\rho(t)\rangle_2],\end{aligned} \tag{S9}$$

* jianshu@mit.edu

where we again used the partial cancellation of the sum terms. The solution reads

$$\langle n(t)\rangle_1 = iJ[1-\langle\rho(0)\rangle_2]t + \langle n(0)\rangle_1 . \tag{S10}$$

Note that in the isolated system, the function $\mathcal{S}[\langle n(t)\rangle_1]$ defined in the main text is constant $\mathcal{S}[\langle n(t)\rangle_1] = J$.

Substituting the obtained results into the definition of $D(t)$ in Eq. (S1), yields the formula

$$D(t) = D_\delta(t) - 2J^2[\mathrm{Re}[\langle\rho(0)\rangle_2] + 2\mathrm{Im}[\langle\rho(0)\rangle_1]^2]t + J(\mathrm{Im}[\langle\rho(0)\rangle_1] + 2\mathrm{Im}[\langle n(0)\rangle_1]). \tag{S11}$$

## II. LIST OF SPATIAL COHERENCES

The diffusivity in Eq. (S11) depends on the initial state through $\langle\rho(0)\rangle_{1,2}$ and $\langle n(0)\rangle_1$. In this section, we provide the explicit expressions for the considered initial states.

### A. Standing Gaussian wave

Substituting the density matrix elements corresponding to the standing Gaussian initial state

$$\psi_n(0) = \frac{\sqrt{2}\cos(kn)}{\sqrt{w\sqrt{\pi}[1+e^{-k^2w^2}]}} \exp\left[-\frac{n^2}{2w^2}\right], \tag{S12}$$

into the definitions in Eq. (S5), yields

$$\langle\rho(0)\rangle_1 \approx \frac{e^{-1/(4w^2)}}{e^{k^2w^2}+1}\left[1+e^{k^2w^2}\cos(k)\right], \tag{S13}$$

$$\langle n(0)\rangle_1 \approx -\frac{1}{2}\frac{e^{-1/(4w^2)}}{e^{k^2w^2}+2}[1+e^{k^2w^2}\cos(k)], \tag{S14}$$

$$\langle\rho(0)\rangle_2 \approx \frac{e^{-1/w^2}}{e^{k^2w^2}+1}\left[1+e^{k^2w^2}\cos(2k)\right], \tag{S15}$$

where we approximated the sums by integrals.

### B. Traveling Gaussian

Similarly, substituting the density matrix elements corresponding to the traveling Gaussian initial state

$$\psi_n(0) = \frac{1}{\sqrt{w\sqrt{\pi}}} \exp\left[-\frac{n^2}{2w^2} + ipn\right], \tag{S16}$$

we get

$$\langle\rho(0)\rangle_1 = \sum_n \rho_{n,n+1} \approx e^{-1/(4w^2)-ip}, \tag{S17}$$

$$\langle n(0)\rangle_1 = \sum_n n\rho_{n,n+1} \approx -\frac{1}{2}e^{-1/(4w^2)-ip}, \tag{S18}$$

$$\langle\rho(0)\rangle_2 = \sum_n \rho_{n,n+2} \approx e^{-1/w^2-2ip}. \tag{S19}$$

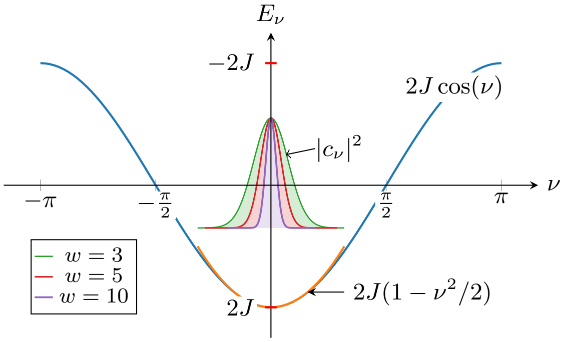


FIG. S1. Dispersion relation, $E_\nu = 2J\cos(\nu)$, and the momentum representation of several Gaussian wave packets with widths $w = 3, 5, 10$. Here, $J < 0$.

## III. MOMENTUM REPRESENTATION

In this section, we invoke the momentum representation of the various initial states to qualitatively explain the diffusivity behavior as a function of initial width and momentum.

### A. Gaussian initial state

The Gaussian initial state is given by

$$\psi_n(0) = \frac{1}{\sqrt{w\sqrt{\pi}}} \exp\left[-\frac{n^2}{2w^2}\right]. \tag{S20}$$

The main text discusses the decay of diffusivity with increasing initial width $w$. Qualitatively, this decay can be understood in terms of the uncertainty principle. The eigenenergies and eigenstates (Bloch states) of the isolated tigh-binding quantum chain are

$$E_\nu = 2J\cos(\nu), \quad \phi_\nu = \frac{1}{\sqrt{2\pi}}e^{in\nu}, \tag{S21}$$

where the quantum number is $\nu \in [-\pi, \pi]$. The squared expansion coefficient of the Gaussian state in terms of the eigenstates is $|c_\nu|^2 \propto \exp(-w^2\nu^2)$. Figure S1 shows the dispersion curve $E_\nu = 2J\cos(\nu)$ and the function $|c_\nu|^2$ for several values of $w$. Note how the increase in $w$ results in shrinking of $|c_\nu|^2$ towards $\nu = 0$. Near $\nu = 0$, the dispersion can be approximated as $E_\nu = 2J\cos(\nu) \approx 2J(1-\nu^2/2)$. Since the wave function is given by $\psi(t) \propto \int_{-\pi}^{\pi} c_\nu \exp(in\nu)\exp(-iE_\nu t)$, increasing $w$ reduces the energy dispersion among the wave packet components, resulting in slower diffusion. Formally, in the limit $w \to \infty$, the wave packet becomes a soliton—a wave packet that retains its shape.

### B. Traveling Gaussian initial state

The traveling Gaussian initial state is given by Eq. (S16). In the main text, we showed that an increase in either the magnitude of the initial momentum $|p|$ or the initial width $w$ leads to diffusivity suppression. The squared expansion

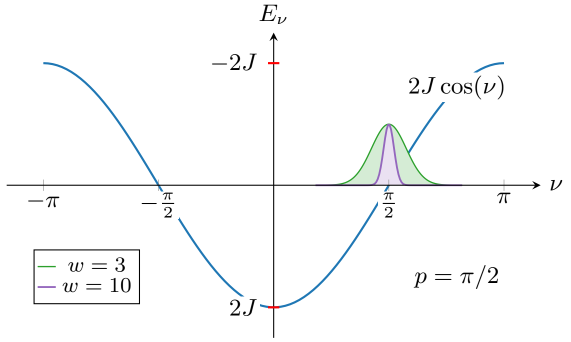


FIG. S2. Dispersion relation, $E_\nu = 2J\cos(\nu)$, and the momentum representation of traveling Gaussian wave packets with widths $w = 3, 10$, and $p = \pi/2$. Here, $J < 0$.

coefficient of the traveling Gaussian state in terms of Bloch states is $|c_\nu|^2 \propto \exp[-w^2(\nu-p)^2]$. Figure S2 shows the dispersion curve $E_\nu = 2J\cos(\nu)$ and the function $|c_\nu|^2$ for several values of $w$. In the previous subsection, we discussed the reason behind the diffusivity rate decrease with increasing $w$.

The reason for the decrease with increasing $|p|$ can be understood by considering the dispersion relation expansion at $\nu = p$

$$E_\nu \approx 2J\left[\cos(p) - \sin(p)(\nu-p) - \frac{\cos(p)}{2}(\nu-p)^2\right]. \quad \text{(S22)}$$

Only quadratic and higher order terms contribute to the wave packet spreading [1]. The coefficient of the quadratic term is $\propto \cos(p)$, which diminishes with increasing $|p|$. At $|p| = \pi/2$, the quadratic term vanishes, and the motion becomes soliton-like.

## IV. DIFFUSIVITY THROUGH THE GREEN-KUBO FORMULA

In this section, we detail the derivation of the diffusivity in the isolated system using the Green-Kubo formula. The dispersion relation and the group velocity are given by

$$E_\nu = 2J\cos(\nu), \qquad v_g = d_\nu E_\nu = -2J\sin(\nu). \quad \text{(S23)}$$

The diffusivity (assuming stationary wave packet's center of mass) is given by the Green-Kubo formula

$$D(t) = \int_0^t \langle v_g(\tau)v_g(0)\rangle\, d\tau = \langle v_g^2\rangle\, t, \quad \text{(S24)}$$

$$\langle v_g^2\rangle = \int_{-\pi}^{\pi} v_g^2 |c_\nu|^2\, d\nu, \quad \text{(S25)}$$

where we used the conservation of group velocity in a closed system, and $c_\nu$ is the overlap integral between the initial state and Bloch state $\nu$

$$|c_\nu|^2 = \left|\frac{1}{\sqrt{2\pi}}\sum_n \psi_n(0)e^{i\nu n}\right|^2. \quad \text{(S26)}$$

### A. Gaussian initial state

For the Gaussian initial state, the expansion coefficient can be calculated by substituting the sum in Eq. (S26) with an integral, resulting in

$$|c_\nu|^2 = \frac{w}{\sqrt{\pi}}e^{-w^2\nu^2}. \quad \text{(S27)}$$

Thus,

$$\begin{aligned}\langle v_g^2\rangle &= \frac{4wJ^2}{\sqrt{\pi}}\int_{-\pi}^{\pi}\sin^2(\nu)e^{-w^2\nu^2}\, d\nu \\ &= -J^2 i e^{-1/w^2}\left[\mathrm{erfi}\left[\frac{1}{w} - i\pi w\right] - \mathrm{erfi}\left[\frac{1}{w} + i\pi w\right]\right] \\ &\quad + 2J^2\mathrm{erf}(\pi w).\end{aligned} \quad \text{(S28)}$$

For consistency with using integrals instead of sums, we assume that $w > 1$. This allows approximating the error functions by $-i$, $i$ and 1, respectively, and we recover the formula from the main text.

$$\begin{aligned}\dot{D}_G = \langle v_g^2\rangle &= 2J^2 - J^2 i(-2i)e^{-1/w^2} \\ &= 2J^2(1 - e^{-1/w^2}).\end{aligned} \quad \text{(S29)}$$

### B. Traveling Gaussian initial state

For the traveling Gaussian initial state, the expansion coefficient reads

$$|c_\nu|^2 = \frac{w}{\sqrt{\pi}}e^{-w^2(\nu-p)^2}.$$

First, we calculate the average group velocity, i.e., the velocity of the center of mass $d_t\langle n\rangle = \langle v_g\rangle$. Like before, we approximate the various error functions to obtain

$$\begin{aligned}\langle v_g\rangle &= \int_{-\pi}^{\pi} v_g|c_\nu|^2\, d\nu = -\frac{2Jw}{\sqrt{\pi}}\int_{-\pi}^{\pi} e^{-w^2(\nu-p)^2}\sin(\nu)\, d\nu \\ &\approx iJe^{-1/(4w^2)}(e^{ip} - e^{-ip}) = -2Je^{-1/(4w^2)}\sin(p),\end{aligned} \quad \text{(S30)}$$

or $\langle n(t)\rangle = -2J\exp[-1/(4w^2)]\sin(p)t$. Similarly,

$$\begin{aligned}\langle v_g^2\rangle &= \frac{4wJ^2}{\sqrt{\pi}}\int_{-\pi}^{\pi}\sin^2(\nu)e^{-w^2(\nu-p)^2}\, d\nu. \\ &\approx \frac{J^2}{2}\left[4 - 2e^{-1/w^2}(e^{2ip} + e^{-2ip})\right] \\ &= 2J^2\left[1 - e^{-1/w^2}\cos(2p)\right].\end{aligned} \quad \text{(S31)}$$

Overall, substituting $\langle n(t)\rangle$ and $\langle v^2\rangle$, we obtain the formula from the main text

$$\begin{aligned}D_T(t) &= \langle v_g^2\rangle\, t - \frac{1}{2}\frac{d\,\langle n(t)\rangle^2}{dt} \\ &= 2J^2[1 - e^{-1/w^2}\cos(2p) - 2e^{-1/(2w^2)}\sin^2(p)]t.\end{aligned} \quad \text{(S32)}$$

## V. DERIVATION – DIFFUSIVITY IN THE PRESENCE OF NOISE (HSR MODEL)

In this section, we derive the diffusivity expression in the presence of noise. Similar to the isolated system, $\rho_{n,n}$ satisfy the differential equation $\dot{\rho}_{n,n} = 2J\text{Im}[\rho_{n-1,n} + \rho_{n+1,n}]$, however $\langle \rho \rangle_l$ [see Eq. (S5)] is no longer conserved. For instance, $\langle \rho \rangle_1$ satisfies

$$\frac{d\langle \rho(t)\rangle_1}{dt} = \sum_n \dot{\rho}_{n,n+1}(t) = -\Gamma \sum_n \rho_{n,n+1} - iJ \sum_n (\rho_{n-1,n+1} - \rho_{n,n} + \rho_{n+1,n+1} - \rho_{n,n+2}). \quad \text{(S33)}$$

where the second term vanishes like in Eq. (S7). Thus, $d_t \langle \rho(t)\rangle_1 = -\Gamma \langle \rho(t)\rangle_1$, such that $\langle \rho(t)\rangle_1 = \langle \rho(0)\rangle_1 \exp(-\Gamma t)$. More generally, for $l \geq 1$,

$$\langle \rho(t)\rangle_l = \langle \rho(0)\rangle_l \, e^{-\Gamma t}. \quad \text{(S34)}$$

Within the HSR model, $\langle n(t)\rangle_1$ satisfies [compare to Eq. (S9)]

$$\frac{d\langle n(t)\rangle_1}{dt} = \sum_n n\dot{\rho}_{n,n+1} = -\Gamma \langle n \rangle_1 + iJ(1 - \langle \rho \rangle_2). \quad \text{(S35)}$$

such that $\mathcal{S}[\langle n(t)\rangle_1] = J - \Gamma \text{Im}[\langle n \rangle_1]$, and

$$\langle n \rangle_1 = \langle n(0)\rangle_1 \, e^{-\Gamma t} + iJ \left[ \frac{1 - e^{-\Gamma t}}{\Gamma} - \langle \rho(0)\rangle_2 \, e^{-\Gamma t} t \right]. \quad \text{(S36)}$$

Collecting all the results, $d_t \langle n^2(t)\rangle$ and $d_t \langle n(t)\rangle$ are given by the expressions

$$\begin{aligned} \frac{d\langle n^2(t)\rangle}{dt} &= 4J\text{Im}[\langle n \rangle_1] + 2J\text{Im}[\langle \rho \rangle_1] \\ &= 4J\text{Im}[\langle n(0)\rangle_1] e^{-\Gamma t} + 2J\text{Im}[\langle \rho(0)\rangle_1] e^{-\Gamma t} \\ &+ 4J^2 \left[ \frac{1 - e^{-\Gamma t}}{\Gamma} - \text{Re}[\langle \rho(0)\rangle_2] e^{-\Gamma t} t \right], \quad \text{(S37)} \\ \frac{d\langle n(t)\rangle}{dt} &= 2J\text{Im}[\langle \rho \rangle_1] = 2J\text{Im}[\langle \rho(0)\rangle_1] e^{-\Gamma t}. \quad \text{(S38)} \end{aligned}$$

The center of mass position is given by

$$\langle n(t)\rangle = \frac{2J}{\Gamma} \text{Im}[\langle \rho(0)\rangle_1](1 - e^{-\Gamma t}), \quad \text{(S39)}$$

where we set $\langle n(0)\rangle = 0$ for simplicity. Expressions for $\langle \rho(0)\rangle_{1,2}$ and $\langle n(0)\rangle_1$ are listed in Sec. II.

[1] R. Robinett, Quantum wave packet revivals, Phys. Rep. **392**, 1 (2004).
